# Supplementary material for: Novel-View Acoustic Synthesis
Source: arXiv:2301.08730 source file (2023-10-24)
Supplement: Supplementary file 1 [file supp.tex]

\setcounter{section}{7}
\setcounter{table}{4}
\setcounter{figure}{4}

\section{Supplementary Material}
In this supplementary material, we provide additional details about:
\begin{enumerate}[itemsep=0mm]
    \item Supplementary video for qualitative assessment of our model’s performance.
    \item Replay-NVAS dataset details (referenced in Sec. 4.1 of the main paper).
    \item SoundSpaces-NVAS dataset details.
    \item Implementation and training details (referenced in Sec. 5.6).
    \item Baseline details (referenced in Sec. 6).
\end{enumerate}

\subsection{Supplementary Video}
This video includes examples for the Replay-NVAS dataset and the SoundSpaces-NVAS dataset as well our model's prediction on both datasets. Listen with a headphone for the spatial sound.

\subsection{Replay-NVAS Dataset Details}

\paragraph{Multi-view camera calibration.} We estimate camera poses with COLMAP~\cite{schoenberger2016sfm} Structure-from-Motion (SfM) framework on each scene separately.
Each scene is filmed with 8 static DSLR cameras and 3 wearable GoPro cameras (the latter are not used in our acoustic synthesis experiments). We first run SfM on the segments of the GoPro recordings where the wearers move significantly; followed by registration of the static camera frames to the model and a final round of bundle adjustment where we enforce constant relative poses between static camera frames taken at the same timestamp. This two-stage procedure greatly reduces the scale of the problem by making SfM focus first on the most diverse part of the data. Upon feature extraction stage, we cull the local features belonging to potentially dynamic object categories (such as people or animals) as detected by Detectron2 instance segmentation \cite{wu2019detectron2}. We then exploit the stationarity of DSLRs by picking a medoid camera pose among the frames filmed by each camera. Finally, we rotate and scale the coordinate system so that Z axis is pointing roughly upwards and scale the scene so that distances between cameras match the approximate field measurements in centimeters. Fig.~\ref{fig:replay_setup} plots all camera coordinates and orientations projected to XY plane. 
\begin{figure}[t]
\centering
\includegraphics[width=0.6\linewidth]{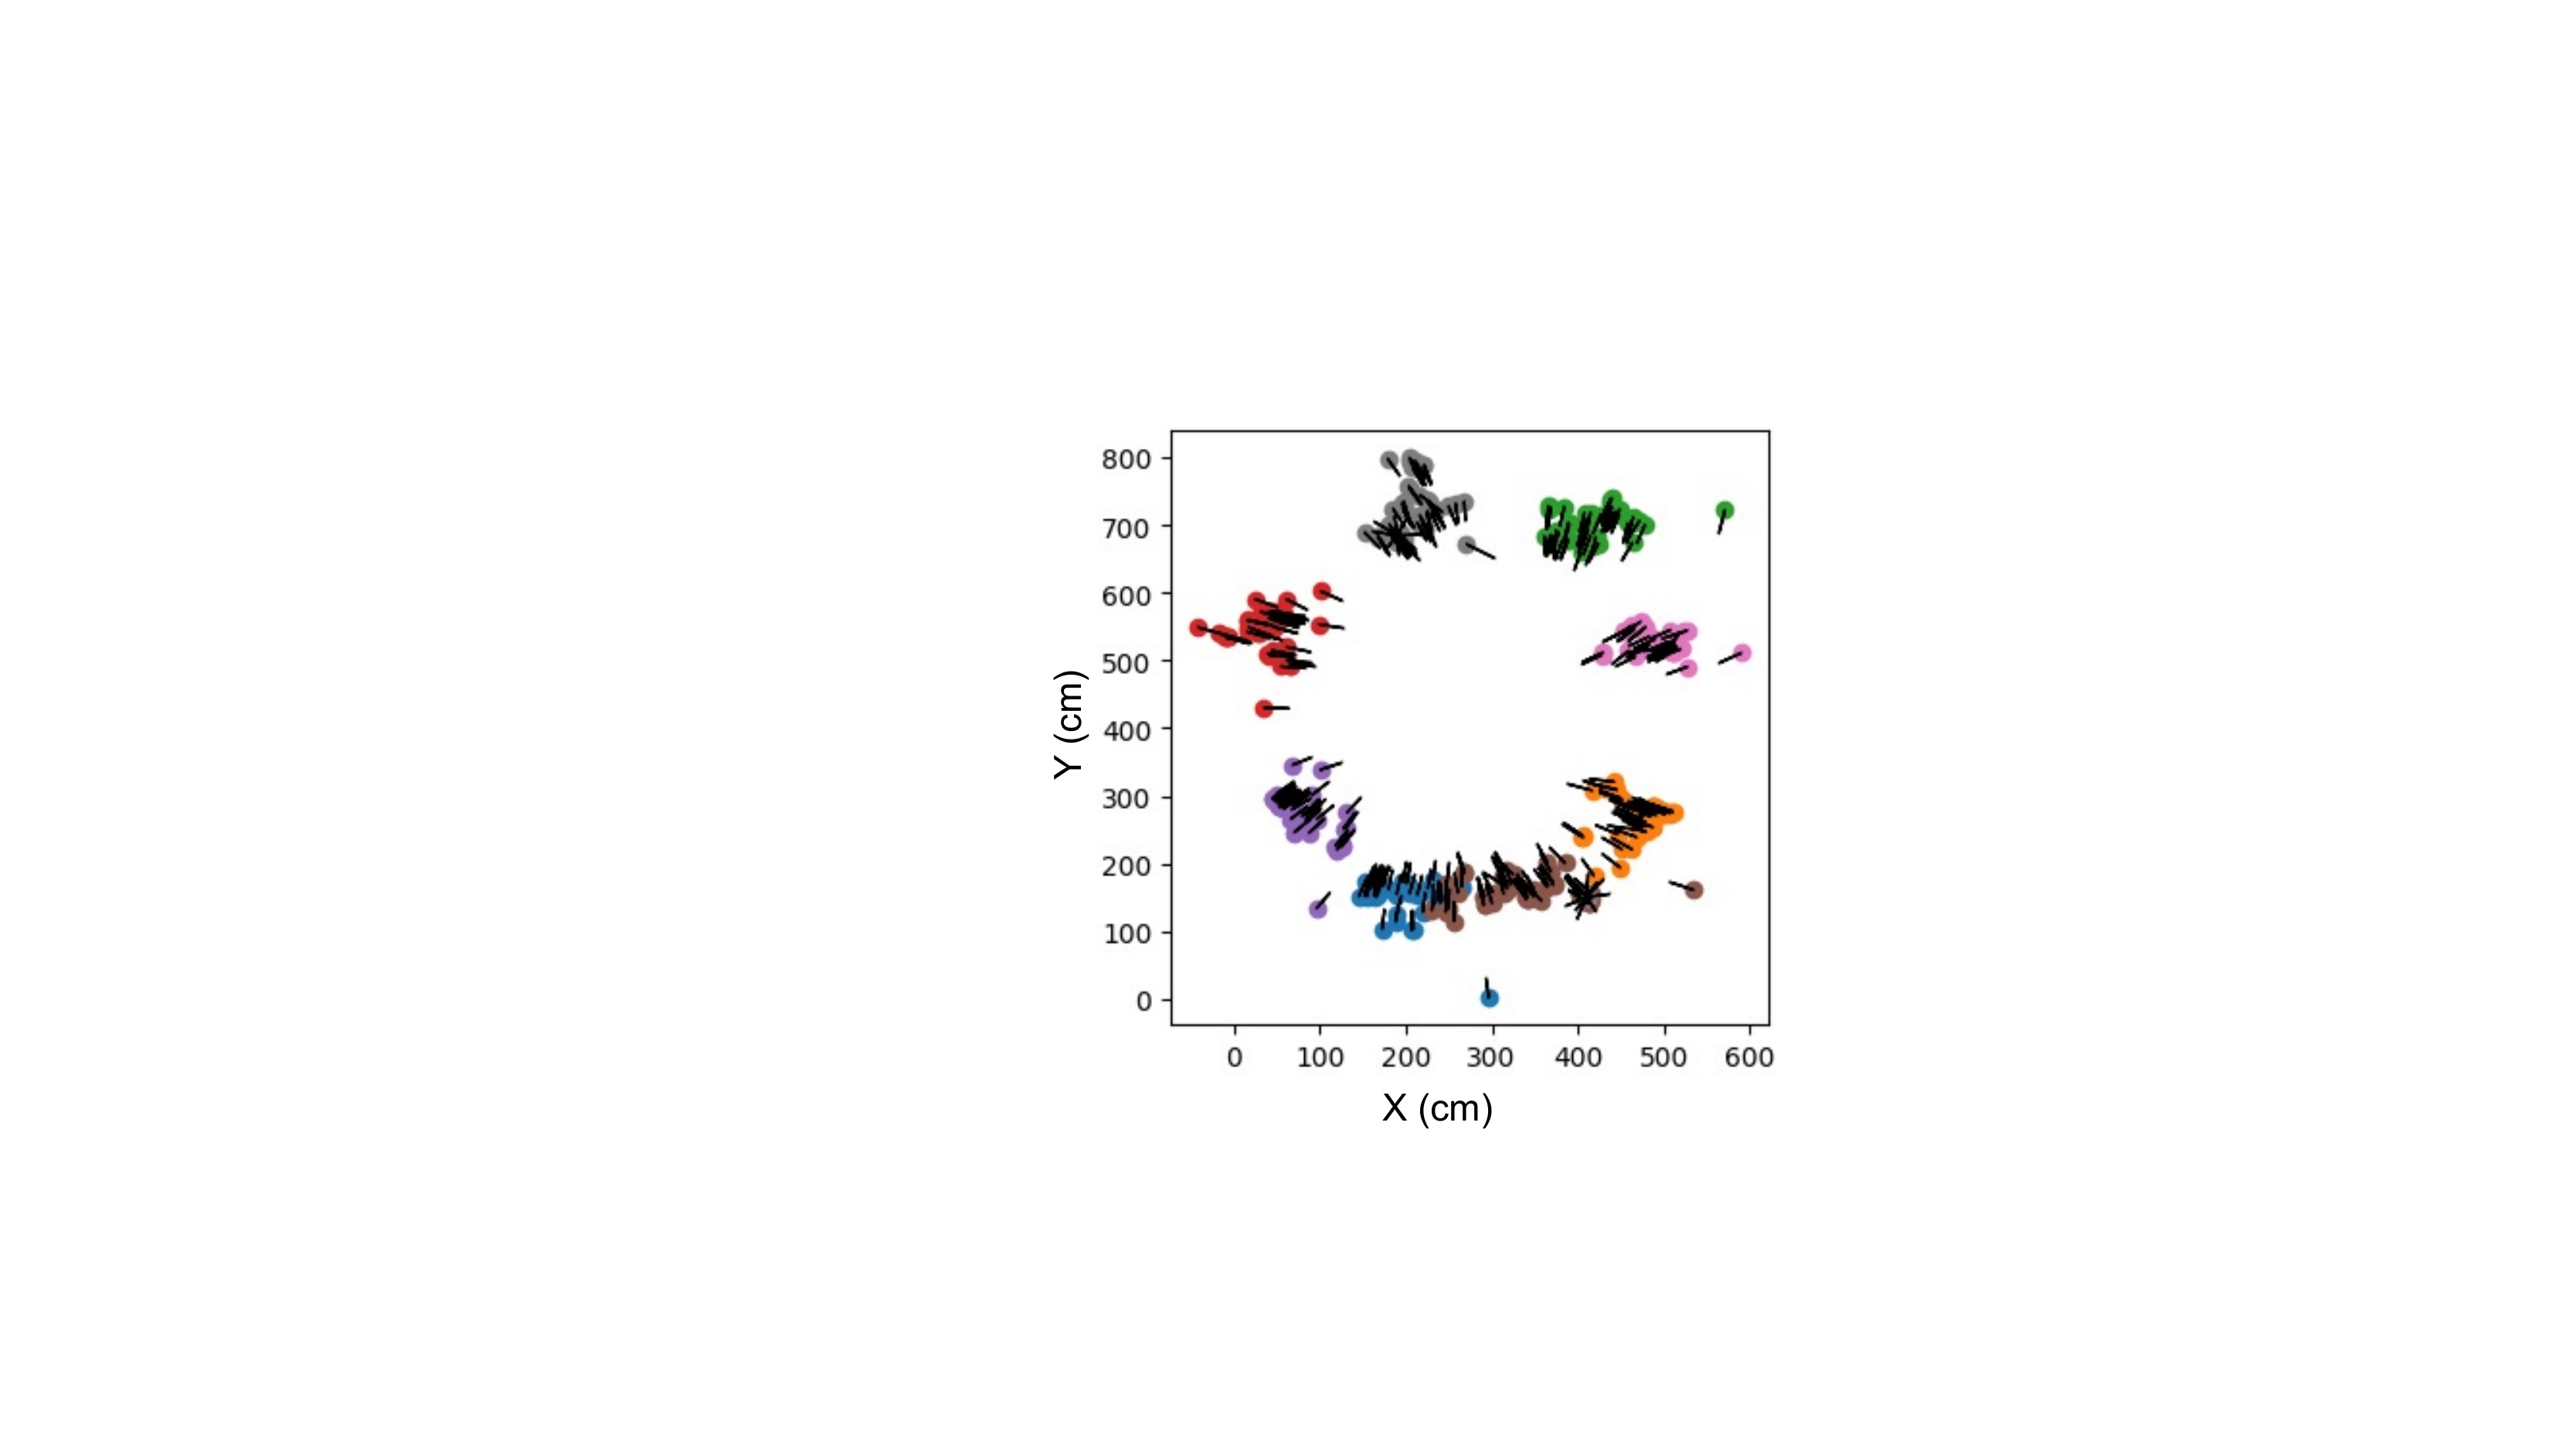}
\vspace{-0.05in}
\caption{Coordinates of static cameras estimated by COLMAP, aggregated over scenes. The same colours correspond to the same camera position estimated from different scenes; they do not collapse to a point since the cameras could be moved between recordings.}
\vspace{-0.15in}
\label{fig:replay_setup}
\end{figure}

\paragraph{Training data construction.}
We temporally align different DSLR videos using the clapper sound that is prominent in the waveform, which gives us synchronized multi-view audio-visual data. However, this data is not directly usable for training because some of it is noisy (e.g., people frequently talking over each other) or silent, which leads to additional learning challenges for the model. Thus, we design an automatic process for filtering out noisy clips. More specifically, we first extract all one-second audio clips of all videos and obtain the corresponding near-range audio clips and bounding boxes for each speaker. As described in Sec. 5.2, we select the active speaker based on the maximum energy of near-range audio with $\Delta t = 0.2$. For a one-second video clip, we obtain 5 candidate bounding boxes. We choose a threshold $\delta\%$ and only keep clips where more than $\delta\%$ of the bounding boxes belong to the same person. We set $\delta$ to $80$. In this way, we keep clips where there is only one dominant speaker talking, and this speaker's bounding box is used as the localization feature $V_L$.

\subsection{SoundSpaces-NVAS Dataset Details}
For the single environment experiment, we use an apartment environment from the Gibson dataset~\cite{xiazamirhe2018gibsonenv}\footnote{\url{http://gibsonenv.stanford.edu/models/?id=Oyens}}. Fig.~\ref{fig:gibson_oyens} shows the mesh of the environment (the ceiling is removed). For the novel environment experiment, we use the public train/val/test splits.

For all images, we render with a resolution of $256 \times 256$ and a field of view of $120$ degrees. We render binaural audio at a sample rate of $16000$.

\begin{figure}
    \centering
    \includegraphics[width=0.6\linewidth]{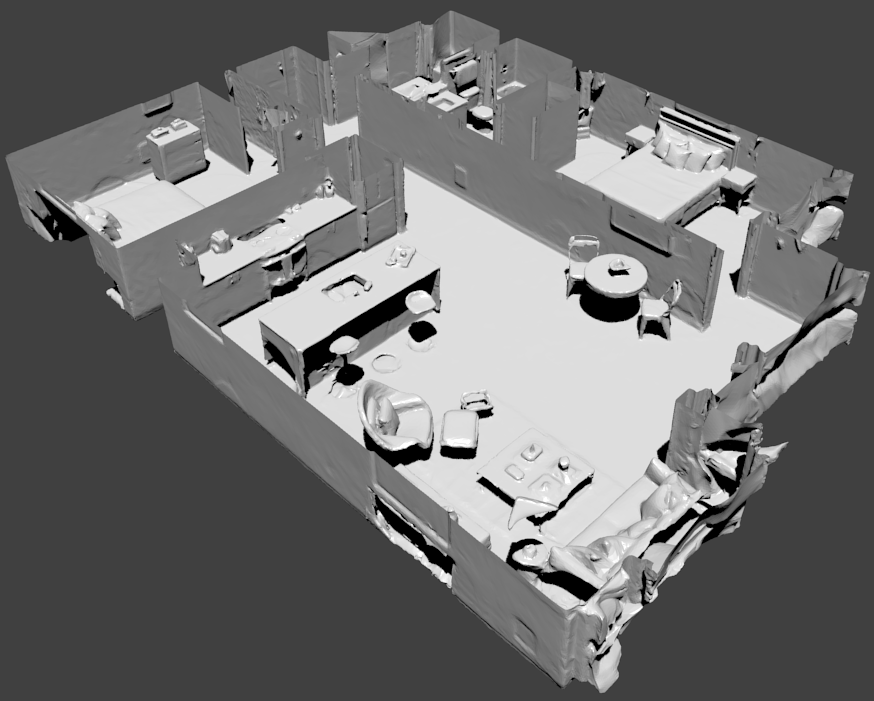}
    \caption{Environment mesh.}
    \label{fig:gibson_oyens}
    \vspace{-0.15in}
\end{figure}

\subsection{Implementation and Training Details}
All audio clips during training are one second long with a sample rate of $16000$. The shape of $A_S$ and $A_T$ is thus $2 \times 16000$. The audio encoder is a conv1d layer that encodes audio from 2 channel (binaural) to latent features of 64 channels, i.e., $A^k_F$ is of shape $64\times 16000$. For acoustic synthesis, we have $M=30$ gated multi-modal fusion layers, which are equally divided into $3$ blocks. In each block, the dilation of the dilated conv1d increases exponentially with base $3$. The kernel size for each dilated conv1d is also $3$. Both the skip and residual layers are conv1d layers with kernel size $1$. The decoder network is a conv1d layer that encodes the latent audio features from $64$ channels back to $2$ channels.

The image resolutions are downsampled to $216 \times 384$ and $256 \times 256$ for Replay-NVAS (downsampled) and SoundSpaces-NVAS respectively. After being processed by a cond1d layer and flattened, the output visual feature $V_F$ is of size $672$ for Replay-NVAS and $512$ for SoundSpaces-NVAS. The fusion layer consists of two fully connected layers with the first output dimension being $512$ and the second being $256$.

We train all models for 1000 epochs on the SoundSpaces-NVAS dataset and for 600 epochs on the Replay-NVAS dataset with a learning rate of $0.001$. We evaluate the checkpoint with the lowest validation loss on the test set. 

\subsection{Baseline Details}
For the Digital Signal Processing (DSP) baseline, we use the head-related transfer function (HRTF) measured by a KEMAR Dummy-Head Binaural Microphone. We apply a Wiener filter~\cite{wiener} to estimate the inverse HRTF. We adjust the gain of the HRTF by performing a binary search on the validation dataset and selecting the best gain value for testing. For the VAM~\cite{chen2022vam} baseline, we take the original model from the paper, and we make minimal modifications by concatenating the visual feature with the target viewpoint pose $P_T$. We train the model with the same hyper-parameters described in the paper until convergence on both datasets.
